# Supplementary material for: Planet as a Brain: Towards Internet of AgentSites based on AIOS Server
Source: arXiv:2504.14411 source file (2025-05-09)
Supplement: Supplementary file 1 [file appendix.tex]

\newpage

\appendix

\section*{\hspace{-4mm} \centering Appendix}
\vspace{3mm}

This appendix provides additional details on the technical implementation of our arXiv template, along with examples to assist users in customizing and utilizing its features effectively. The template leverages modern LaTeX packages such as \texttt{geometry}, \texttt{fontspec}, and \texttt{microtype} to ensure precise control over layout and typography, while advanced functionalities like automated metadata generation and multi-column layouts are designed for ease of use. Notably, Qwen and DeepSeek contributed significantly to optimizing code efficiency and refining design elements, particularly in handling complex equations and improving figure/table placement. Below are sample code snippets demonstrating key features, including title page setup, multi-column formatting, and bibliography management. Users are encouraged to experiment with these examples to tailor the template to their specific needs while maintaining a professional and visually appealing presentation.
